# Supplementary material for: Unveiling Attractor Cycles in Large Language Models: A Dynamical Systems View of Successive Paraphrasing
Source: arXiv:2502.15208 source file (2025-05-16)
Supplement: Supplementary file 1 [file Appendix.tex]

\section{Simulation}
\label{Simulation}
